# Supplementary material for: How superfluid vortex knots untie
Source: arXiv:1507.07579 source file (2015-07-27)
Supplement: Supplementary file 1 [file supplemental_arxiv.pdf]

# How superfluid vortex knots untie: supporting materials


Dustin Kleckner,[1] Louis H. Kauffman,[2] and William T. M. Irvine[1]

[1] *James Franck Institute and Department of Physics, The University of Chicago, Chicago, IL 60637, USA*

[2] *Department of Mathematics, Statistics and Computer Science, University of Illinois at Chicago, Chicago, IL, 60607, USA*


## SIMULATION DETAILS

The time evolution of the superfluid wavefunction was computed by numerically integrating the Gross Pitaevskii equation using a spit-step spectral method along the lines of [1, 2]. For simulations with mean radius $r_0/\xi = \{15, 25\}$, we use a grid size of $\Delta x = 0.5\xi$, a simulation time-step of $\Delta t = 0.02$, and save the traced vortex paths at an interval of $\Delta T = 1$. For simulations with $r_0 = 50\xi$, we compute a coarser simulation with $\Delta x = 1\xi$, $\Delta t = 0.1$, and $\Delta T = 4$. A small number of simulations of the same sized knot at different resolutions was used to confirm that the coarser simulations do not significantly affect the computed length and helicity of the vortex as it unties (the noise in these computed quantities does increase, but we do not observe systematic differences). The total size of the periodic simulation box was $L/\xi = \{128, 192, 384\}$ for $r_0/\xi = \{15, 25, 50\}$, respectively. Occasionally, small vortex rings ejected from the untying vortices interact with their periodic partners by traversing the boundary; in general this only happens after the vortices have untied. To ensure that the size of the box does not affect the behavior of the knot, we have simulated the same knot in several differently sized periodic volumes; we find that the behavior of the knot is virtually identical so long as it is spaced more than a few $r_0$ from its periodic partner (in practice, the most complex knots have a maximum extent of only around half the length of edge of the simulation box).

## INITIAL STATE CONSTRUCTION

The phase fields for the initial states were generated by brute force integration of a Biot-Savart generated flow field, $\boldsymbol{u}_{BS}$, which is related to the phase-gradient via the relationship:

$$\nabla\phi(\boldsymbol{x}) = \boldsymbol{u}_{BS}(\boldsymbol{x}) \tag{1}$$

This method is described in more detail in [2]. An example an initial phase field is shown in Figure 1**e** of the main text. The shape of ideal knots for different topologies were obtained from [3], and were initially generated via the SONO method [4].

## CALCULATION OF HELICITY AND VORTEX ENERGY

For each saved time-step, a polygonal representation of the vortex shape is obtained by tracing the phase defects in the superfluid wavefunction with a resolution set by the simulation grid (typically $\gtrsim 10^3$ points total). Additionally, a phase normal, $\hat{\boldsymbol{\phi}}$, is computed for each point on the vortex by finding the direction of zero phase which is perpendicular to the vortex path.

As stated in the main text, we compute the centerline helicity in the dimensionless form:

$$h = \sum_{i \neq j} Lk_{ij} + \sum_i Wr_i \tag{2}$$

Although this can be computed directly from the polygonal paths, this method requires special considerations for dealing with linking across periodic boundaries. Alternatively, we may note that a surface of constant phase defines a 'Seifert framing' for each knot/link obeying $h + \sum_i Tw_{\phi,i} = 0$ [5], where $Tw_{\phi,i}$ is the twist of the phase normal about the vortex path:

$$Tw_{\phi,i} = \oint_{\mathcal{C}_i} d\boldsymbol{\ell} \cdot \hat{\boldsymbol{\phi}} \times \partial_s \hat{\boldsymbol{\phi}}, \tag{3}$$

where $\mathcal{C}_i$ refers to closed vortex path $i$ and $\partial_s$ is a path-length derivative. As the total twist can easily numerically integrated from the vortex path and phase normal, it provides an efficient method for computing centerline helicity. We have numerically confirmed that this method provides results equal to direct computation of linking and writhe, up to numerical precision.

The energy associated with the vortices in the superfluid (as opposed to sound waves) is computed from the 'path inductance' [6], $\mathcal{E}_{ij}$, of the vortex centerlines:

$$E_v = \frac{\rho\Gamma^2}{2} \sum_{ij} \mathcal{E}_{ij} \tag{4}$$

$$\mathcal{E}_{ij} = \frac{1}{4\pi} \oint_{\mathcal{C}_i} \oint_{\mathcal{C}_j}^{|\vec{r}_i - \vec{r}_j| > \frac{\xi}{2}} \frac{d\vec{r}_i \cdot d\vec{r}_j}{|\vec{r} - \vec{r}_j|} + \delta_{ij} \frac{2-\alpha}{2\pi} L_i, \tag{5}$$

where $\alpha \cong 1.615$ is a dimensionless correction factor chosen to obtain the correct value for the energy of a vortex

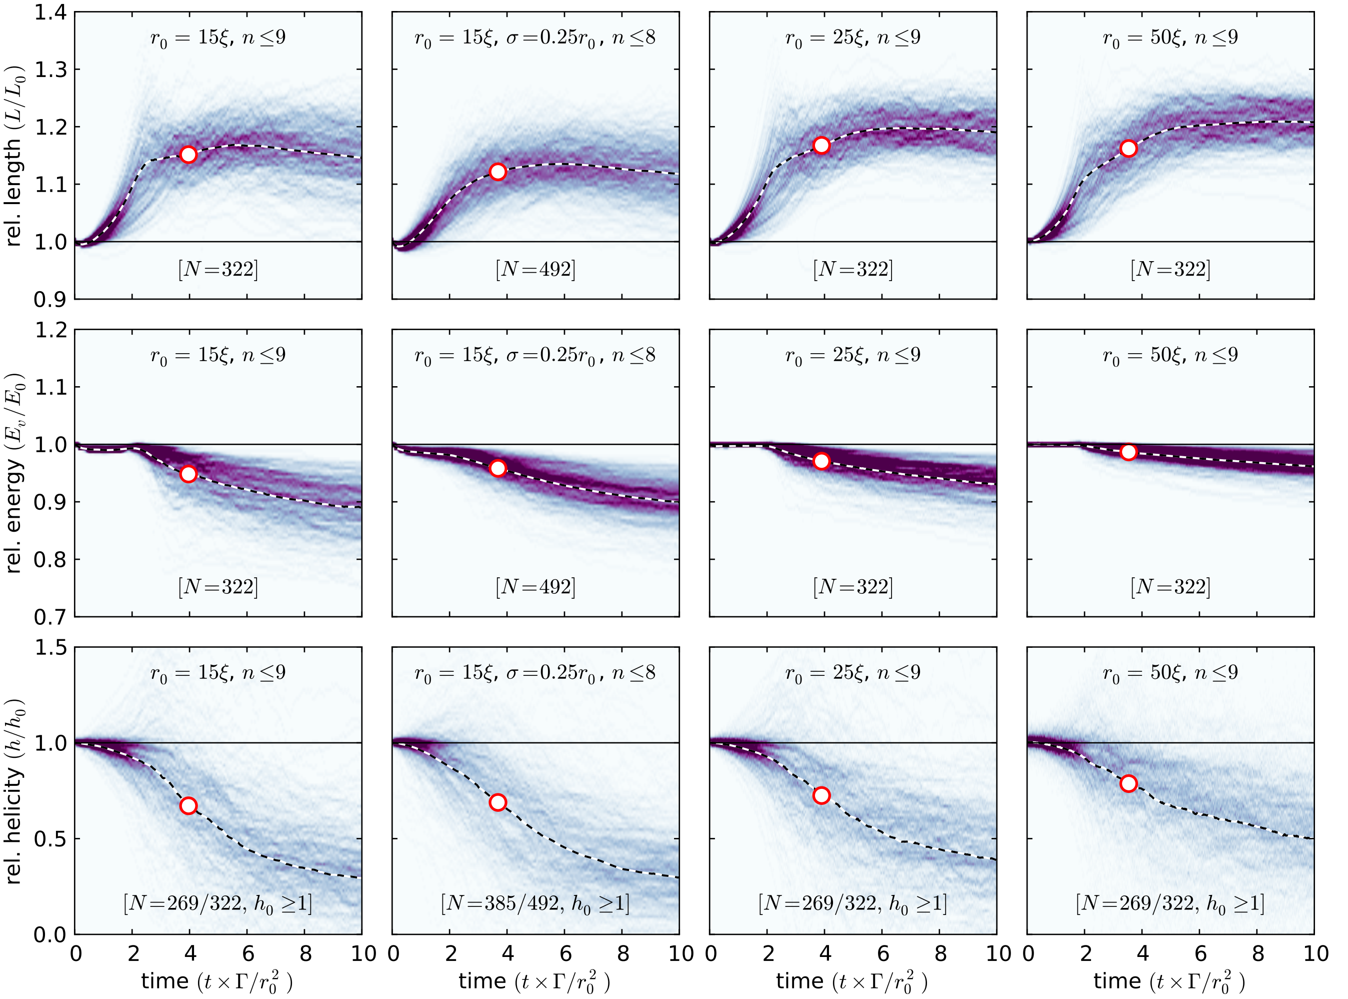


FIG. S1: Histograms of the length, energy, and helicity (top to bottom) as a function of time for each group of simulations (smallest to largest knots from left to right). The dashed line indicates the average value of each time; the red circle indicates the average moment that the knots become untied. For the helicity histograms, only those simulations with initial helicity $h \geq 1$ are included.

| | $r_0 = 15\xi$, ideal, $n \leq 9$ | $r_0 = 25\xi$, ideal, $n \leq 9$ | $r_0 = 50\xi$, ideal, $n \leq 9$ | $r_0 = 15\xi$, $\sigma = 0.25r_0$, $n \leq 8$ |
|---|---|---|---|---|
| Unknotting time: $t \times \Gamma/r_0^2$ | $4.0^{+1.8}_{-1.2}$ | $3.9^{+2.0}_{-1.3}$ | $3.5^{+2.0}_{-1.3}$ | $3.7^{+2.2}_{-1.4}$ |
| Length: $\langle \Delta L/L_0 \rangle$ | +18.5% | +19.3% | +18.0% | +13.6% |
| Helicity: $\langle \Delta h \rangle / \langle h_0 \rangle$ | −38.9% | −31.7% | −25.7% | −34.4% |
| Energy: $\langle \Delta E_v/E_0 \rangle$ | −4.86% | −2.61% | −1.25% | −3.87% |
| Absolute energy: $\langle \Delta E_v \rangle / \left(\rho \Gamma^2 \xi\right)$ | −7.18 | −7.43 | −8.40 | −5.45 |
| Abs. energy, only $n = 8$: $\langle \Delta E_v \rangle / \left(\rho \Gamma^2 \xi\right)$ | −6.59 | −7.04 | −7.80 | −5.93 |

TABLE SI: Average change in various quantities at the moment that the vortex knots first untie. The specified range for the unknotting time indicates the $1\sigma$ bounds of a log-normal fit to the histogram of values (see Figure 3**a-d**). The mean relative helicity change is computed slightly differently than the other quantities, to prevent states from zero or near-zero initial helicity from skewing the results. The last two rows give the absolute change in the energy, in non-dimensional units, and the last column gives values only for topologies with initial crossing number $n = 8$.

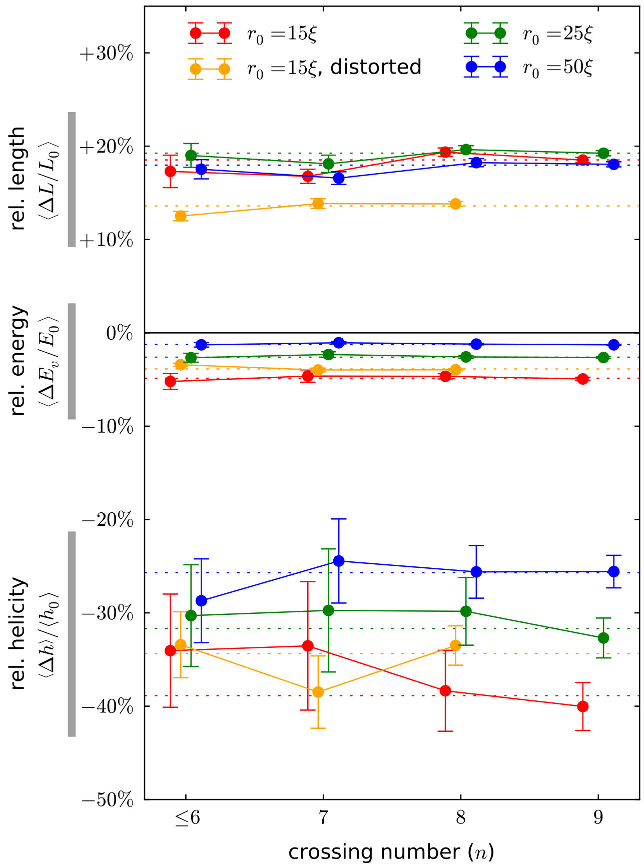


FIG. S2: The average change in length, energy, and helicity as a function of crossing number for each group of simulations. In each case, the change is taken between the initial state and the moment of untying. Error-bars indicate the uncertainty in the average. Topologies with crossing number $n \leq 6$ are grouped together to obtain adequate statistics. In every case, there is no significant trend observed as a function of crossing number.

ring in the GPE [7]. To account for the periodic nature of the simulations, the cross inductance is included for a $3 \times 3 \times 3$ periodic array of vortex paths. (Including more periodic copies improves the accuracy of the calculation, but the difference is typically only a small fraction of a percent). Note that the total energy in the superfluid is conserved, so a reduction in vortex energy corresponds to an increase in the energy in sounds waves, which can be seen to be created during each reconnection event. The vast majority of energy changes in the vortices is seen to occur during reconnection events; otherwise the computed energy is nearly constant.

## VORTEX LENGTH, ENERGY, AND HELICITY

As described in the main text, the behavior of unknotting vortices is described by several generic features, regardless of knot scale, complexity, or shape distortions. Figure S1 shows histograms of the evolution of length, energy, and helicity for each group of simulations, and Table SI shows the average change in these quantities at the moment that the knots first become untied. Figure S2 shows the average change in these quantities as a function of crossing number. For all three measures, the relative change in these quantities appears to be unaffected by topological complexity: very tangled vortex lines behave (on average) similarly to simple links and knots.

The most notable geometric feature of the evolution of vortex knots is that they stretch: on average, the vortex lines are about 20% longer when they finish untying. Interestingly, this stretching stops abruptly after the knot is untied. This evolution appears to be caused by the tendency of a concentrated region of vorticity to expand. For unknotted vortices, individual vortex rings can separate without stretching; this is not possible for a collection of tangled vortex lines.

Uniform stretching would produce an increase in the energy of the vortices, and so there must also be a geometric rearrangement of the vortex lines in order to conserve energy. As previously observed for the evolution of simple knots in classical fluid vortices, this conservation is obtained by forming closely spaced anti-parallel regions, which have a lower energy density [6]. Eventually, these regions become close enough that they drive reconnection events. Thus, taken as a whole, vortex topology drives stretching, which in turns produces reconnections which eventually untie the vortex knots.

We note that this feature can also be reproduced by running the simulations backwards. Thus the ideal knots are near to a local minimum of vortex length in the world line of the superfluid wavefunction.

The total dissipation in vortex energy is relatively small, $\Delta E_v \lesssim 0.05 E_0$, with relatively less dissipation for larger vortex knots following an approximate $\Delta E_v \propto r_0^{-1.0}$ trend. Alternatively, we note that the *absolute* change in energy is roughly the same for all simulation groups (up to an apparent logarithmic correction due to the finite core). This aries because the vortex energy is only dissipated during reconnection events, and the amount dissipated is primarily by the number of reconnections (rather than global or topological features). The absolute dissipation shows a dependance on crossing number, unlike other geometric features, but this dependance disappears when rescaled by the initial energy, which is also higher for more complicated knots (which are larger/longer for the same 'rope scale', $r_0$).

The dissipation of helicity is also affected by scale, following an approximate $\delta E_v \propto r_0^{-0.5}$ trend. This is in agreement with a similar observation of better helicity conservation at larger scales previously observed for trefoil knots in a different geometry [2]. The difference in scaling between helicity and energy is reflective of the different character of these two quantities: energy is dom-

inated by local arrangements, while helicity is sensitive to the global topology and coiling of the vortex lines.

## IDENTIFICATION OF VORTEX TOPOLOGY

To identify the topology of the superfluid vortices at each time-step, the polygonal vortex representation is first reduced to the minimum possible number of points possible without changing the topology (unknots are also removed at this stage, if they are not threaded by any other vortex lines). Once the vortices are reduced, they are projected into an arbitrary 2D plane and the projected crossings and their handedness are identified; the HOMFLY-PT polynomial is created directly from this crossing list. This polynomial is compared to an internally generated database of HOMFLY-PT polynomials for all topologies (including chiral pairs, oriented links, and disjoint and compound knots/links) with a minimal crossing number of $n \leq 10$. This database was generated starting from the crossing diagrams obtained from [8, 9]. The equivalence of oriented links was determined by assuming all orientational permutations with identical HOMFLY-PT polynomials are topologically equivalent. The HOMFLY-PT polynomial of disjoint and compound topologies was computed algebraically from the HOMFLY-PT polynomials of their components. We do not treat configurations with extra unknots to be distinct topologies, and do not distinguish between disjoint and compound topologies. (We note that disjoint knots are rarely observed in the decay pathways, and are furthermore difficult to distinguish from compound knots via HOMFLY-PT polynomials if unknots are also present.) There exist several knots/links with identical HOMFLY-PT polynomials for $n \geq 9$, but we do not encounter any of these in the observed pathways for knots starting with $n \leq 8$, which were used to compute decay pathways.


[1] Proment, D., Onorato, M. & Barenghi, C. Vortex knots in a bose-einstein condensate. *Phys. Rev. E* **85**, 1–8 (2012).

[2] Scheeler, M. W., Kleckner, D., Proment, D., Kindlmann, G. L. & Irvine, W. T. M. Helicity conservation by flow across scales in reconnecting vortex links and knots. *PNAS* **111**, 15350–15355 (2014).

[3] The knot atlas: Ideal knots. URL `http://katlas.math.toronto.edu/wiki/Ideal_knots`.

[4] P Pieranski. In search of ideal knots. In Stasiak, A., Katritch, V. & Kauffman, L. H. (eds.) *Ideal Knots* (World Scientific, 1998).

[5] Akhmet'ev, P. & Ruzmaikin, A. Borromeanism and bordism. In Moffatt, H. K., Zaslavsky, G. M., Comte, P. & Tabor, M. (eds.) *Topological Aspects of the Dynamics of Fluids and Plasmas*, no. 218 in NATO ASI Series, 249–264 (Springer Netherlands, 1992).

[6] Kleckner, D. & Irvine, W. T. M. Creation and dynamics of knotted vortices. *Nat. Phys.* **9**, 253–258 (2013).

[7] Donnelly, R. J. Vortex rings in classical and quantum systems. *Fluid Dyn. Res.* **41**, 051401 1–31 (2009).

[8] Cha, J. C. & Livingston, C. KnotInfo: Table of knot invariants. URL `http://www.indiana.edu/~knotinfo`.

[9] Cha, J. C. & Livingston, C. LinkInfo: Table of knot invariants. URL `http://www.indiana.edu/~linkinfo`.
